# Supplementary material for: Predicting polymorphism in molecular crystals using orientational entropy
Source: arXiv:1806.06006 ancillary file (2018-06-15)
Supplement: Supplementary file 1 [file supplemental_material.pdf]

Supplemental information to:
# PREDICTING POLYMORPHISM IN MOLECULAR CRYSTALS USING ORIENTATIONAL ENTROPY

Pablo M. Piaggi and Michele Parrinello

June 15, 2018

## 1 Urea

In Figure SI-1 we show the two biased collective variables (CVs) $s_{\theta_1}$ and $s_{\theta_2}$ as a function of simulation time. The angles $\theta_1$ and $\theta_2$ for the two CVs are also depicted in this figure.

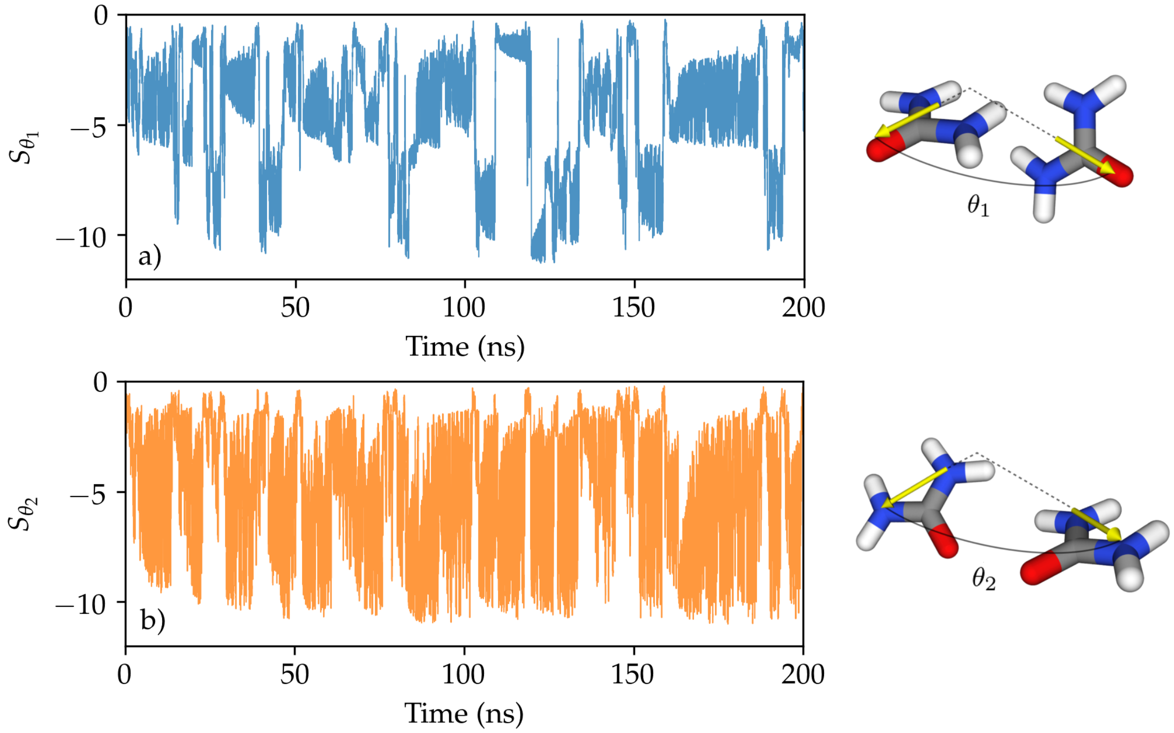


Figure SI-1: Biased CVs a) $s_{\theta_1}$ and b) $s_{\theta_2}$ as a function of simulation time for urea at 450 K. The definition of the angles $\theta_1$ and $\theta_2$ for the two CVs are also depicted.

### 1.1 Urea form B

We compare the rotation of urea molecules around the C-O axis in form I and form B. To this end we calculate the autocorrelation function of $\langle \hat{\mathbf{v}}(0) \cdot \hat{\mathbf{v}}(t) \rangle$ where $\hat{\mathbf{v}}(t)$ is

the unit vector that characterizes the orientation in space of the N-N bond of each urea molecule at time $t$. We show the results in Figure SI-2 a). We also calculate the free energy as a function of the rotation angle around the C-O axis. We compare the free energy for forms I and B in Figure SI-2 b). The barrier in form B is significantly lower than in form I.

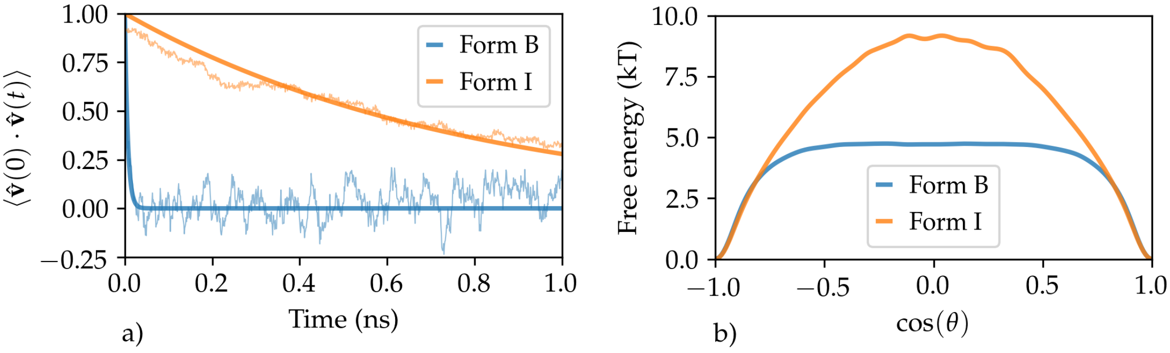


Figure SI-2: a) $\langle \hat{\mathbf{v}}(0) \cdot \hat{\mathbf{v}}(t) \rangle$ autocorrelation function and b) Free energy profile with respect to $cos(\theta)$ for forms I and B.

Form B of urea experiences a phase transition while cooling from room temperature. In order to study the transition from the high temperature form to the low temperature one, we quench the system from 300 K to 0 K in 100 ns and then we increased the temperature back to 300 K in the same time span. We use the peak of the x-ray diffraction (XRD) pattern corresponding to $2\theta = 29.5$ using $\lambda = 1.5406$ Å as order parameter to track the evolution of the system. This particular XRD peak has a high intensity in the low temperature form and a low intensity in the high temperature one. The intensity of this XRD peak during the simulation is shown in Fig. SI-3. From this figure we observe a small yet non negligible hysteresis in the behavior of the order parameter as the temperature is raised or lower. It is useful to calculate the susceptibility $\chi$, that is to say the standard deviation of the order parameter, as a function of temperature. As seen in the inset of Fig. SI-3 this quantity exhibits a peak in the transition region. We therefore identify the transition temperature as being in the interval from 125 K to 200 K.

We thought useful to report the XRD pattern of form B at 300 K such that experimental results can be compared directly. This is shown in Figure SI-4. The XRD pattern was computed using $\lambda = 1.54059$ Å and $\lambda = 1.54432$ Å with relative intensities 1 and 0.5, respectively.

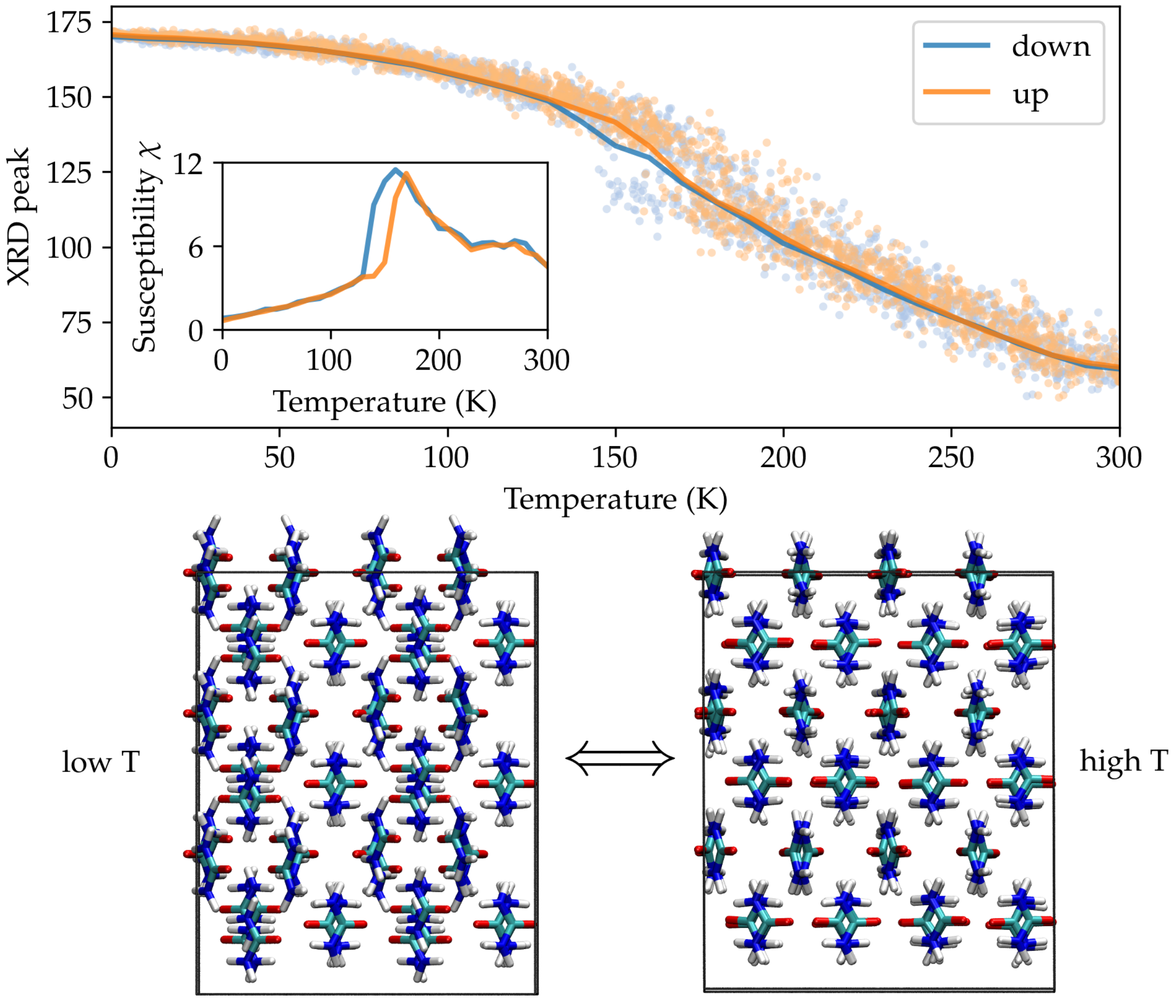


Figure SI-3: Interconversion between low and high temperature of urea polymorph B. Evolution of one of the XRD peaks used as order parameter as a function of temperature (see text for details). The points labeled as up and down correspond to trajectories in which the temperature was raised and lowered, respectively. The solid lines are shown to guide the eyes. Snapshots of the low and high temperature forms are shown.

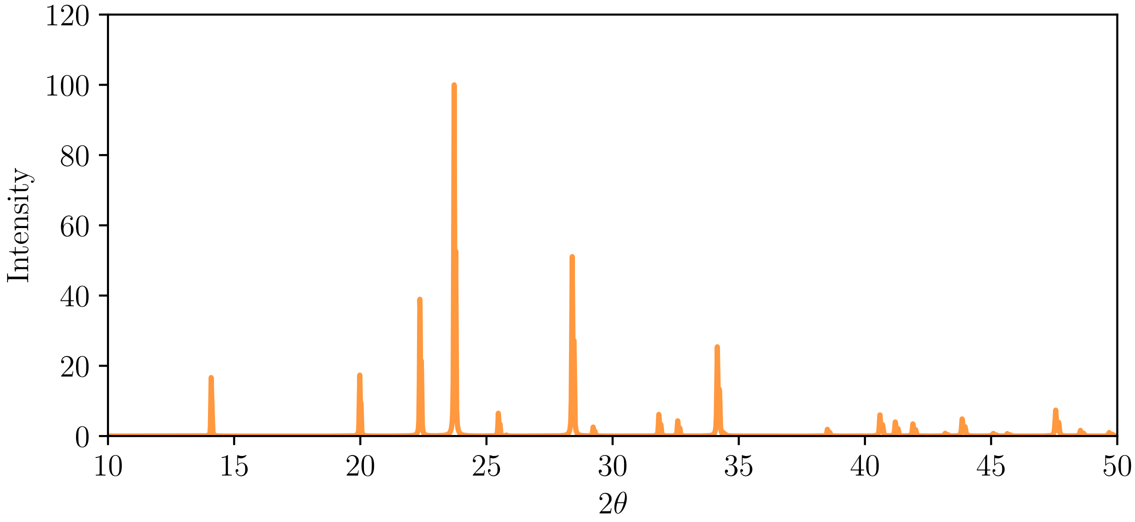


Figure SI-4: XRD pattern of urea polymorph B at 300 K.

## 2 Naphthalene

In Figure SI-5 we show the two biased CVs $s_{\theta_1}$ and $s_{\theta_2}$ as a function of simulation time. The angles $\theta_1$ and $\theta_2$ for the two CVs are also depicted in this figure.

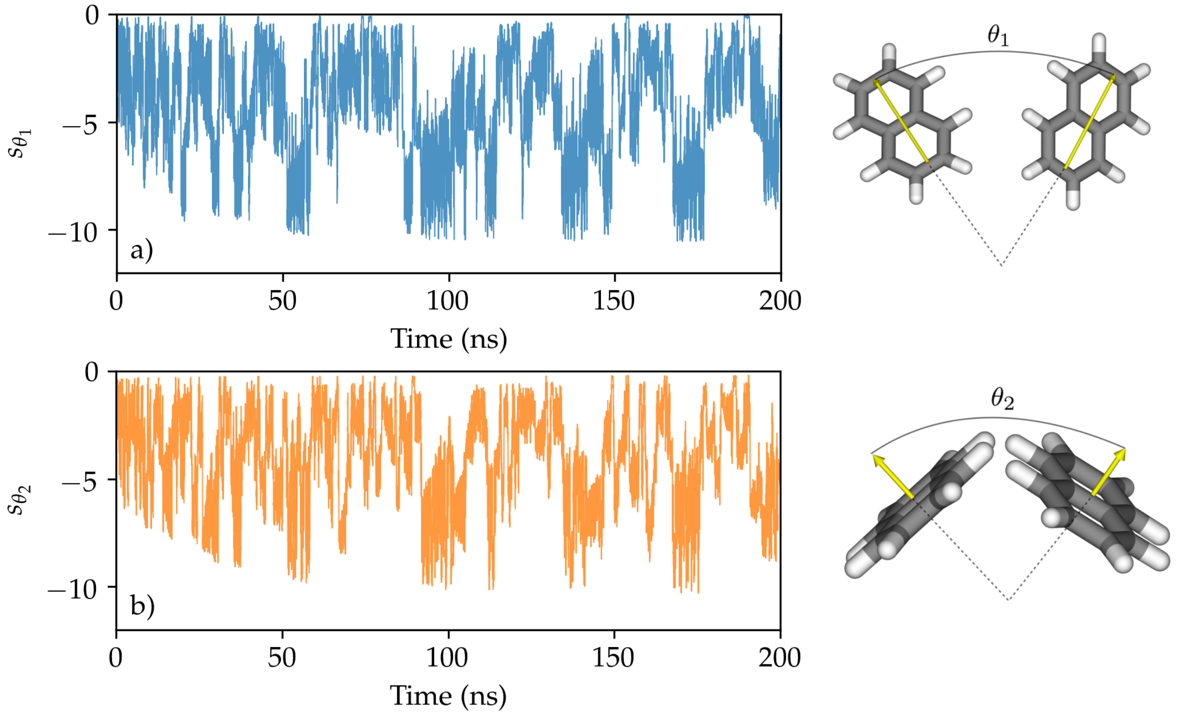


Figure SI-5: Biased CVs a) $s_{\theta_1}$ and b) $s_{\theta_2}$ as a function of simulation time for naphthalene. The definition of the angles $\theta_1$ and $\theta_2$ for the two CVs are also depicted.

We perform a clustering of the trajectory of naphthalene at 300 K using the distance defined in Eq. 4 of the main part. The results of the clustering are shown in Figure SI-6. The algorithm identifies five different clusters. Two of them correspond to partially ordered structures. The other clusters correspond to form I, form A and the liquid.
As in the case of urea polymorph B, here we report the XRD pattern of naphthalene form A. This is shown in Figure SI-7. The XRD pattern was computed using the same wavelengths described above.

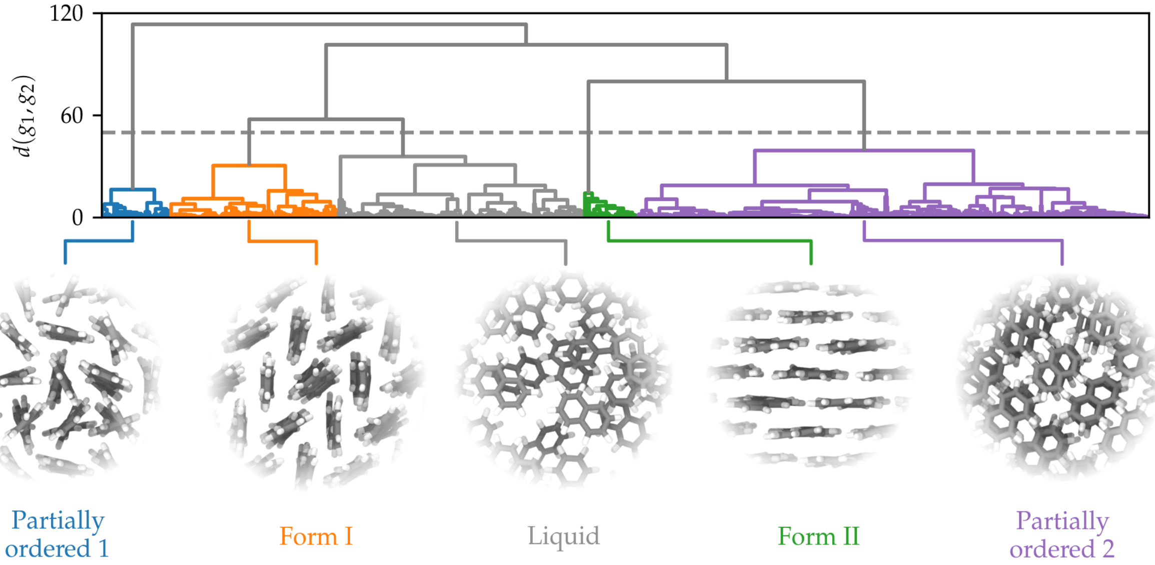


Figure SI-6: Tree diagram resulting from the clustering of the trajectory of naphthalene at 300 K. Configurations at 300 K for the clusters are shown.

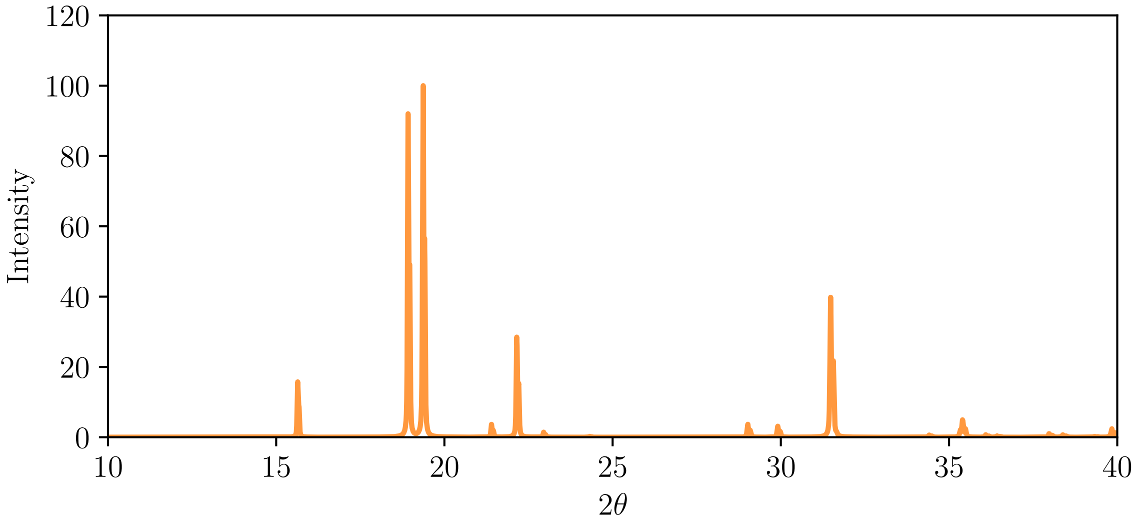


Figure SI-7: XRD pattern of naphthalene polymorph A at 300 K.
